# Supplementary material for: Clathrate Structure of Fullerite C60
Source: arXiv:2107.05909 source file (2021-07-28)
Supplement: Supplementary file 1 [file SupportingInformation_v3.pdf]

## Supporting Information

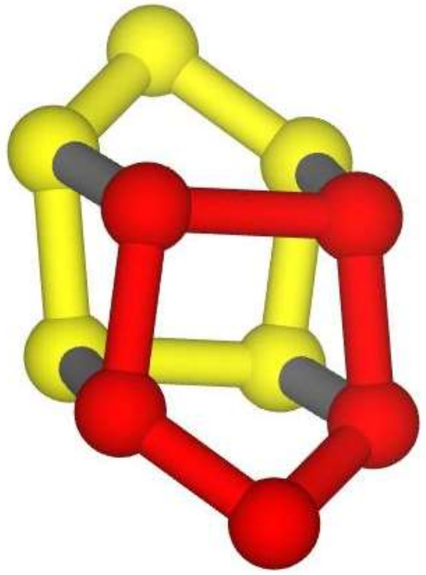

Figure S1: Highlight of double 5/5 2+3 cycloaddition bonding between pentagons of $C_{60}$ neighboring molecules (depicted with yellow and red colors). Intermolecular bonds are colored in grey.

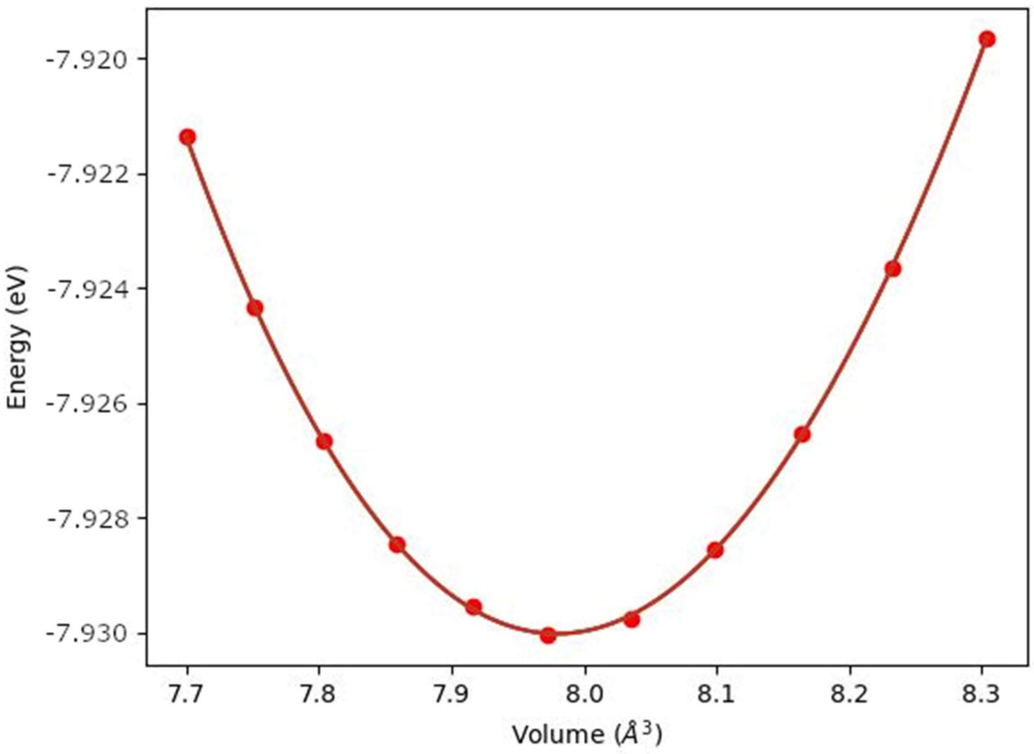


Figure S2: The total energy per atom for the $C_{60}$-based clathrate as a function of volume per atom.

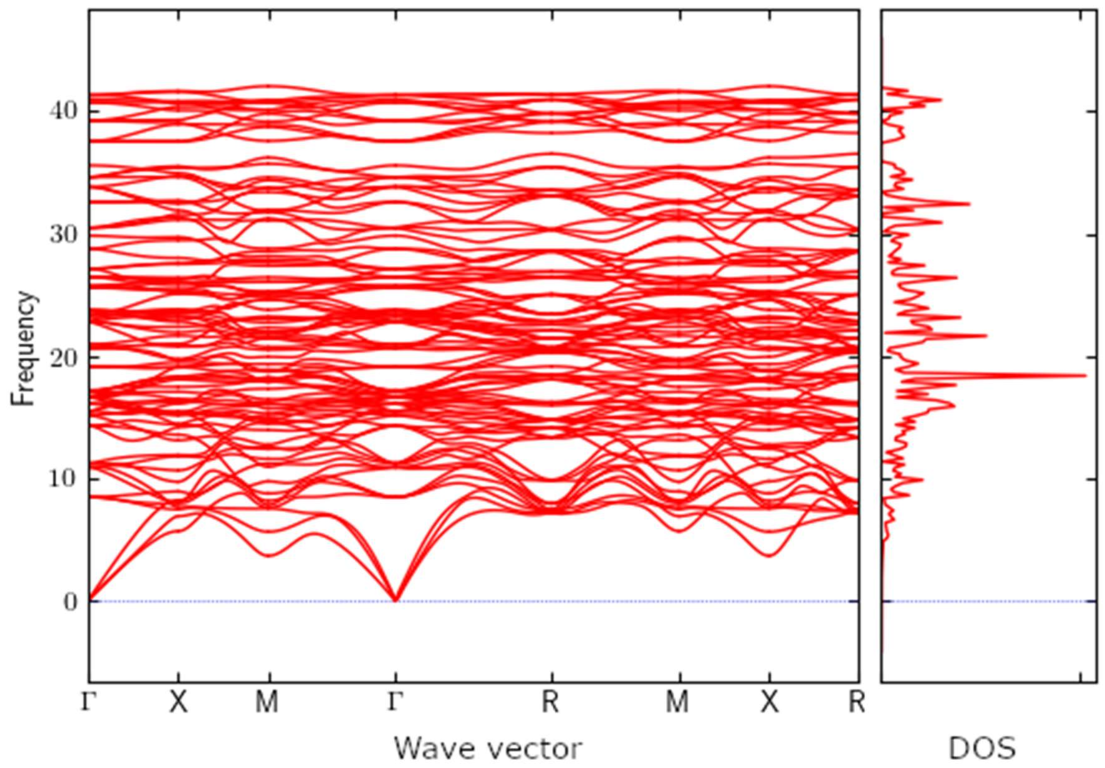


Figure S3: Phonon dispersion (left panel) and phonon density of states (right panel) of the $C_{60}$-based clathrate.

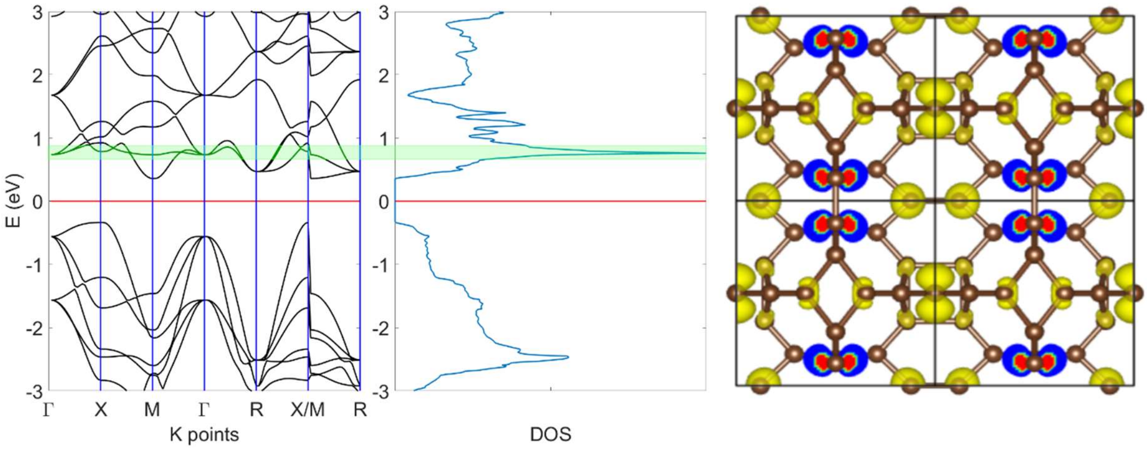


Figure S4: The electronic band structure (left panel), the electronic density of states, DOS, (center panel) and the partial charge density around the DOS peak (right panel), for the C60-based clathrate. Red lines indicate the Fermi level. The energy range where the partial charge density was integrated is the green-colored region shown in the left and center panels. Isosurface plots of the partial charge density are superposed with ball-and-stick models in the (100) crystallographic plane and the isosurface value is $4.0 \times 10^{-3}$ e/Å$^3$.

**Table S1:** Optimized atomic positions of the $C_{60}$-based clathrate structure in the P$m\bar{3}$ simple cubic cell with lattice parameter 6.17Å, using HSE06-6-31G(d,p) as implemented in gaussian09.

| atom | x | Y | z | Wyckoff Position |
|---|---|---|---|---|
| C1 | 0.50000 | 0.34929 | -0.14142 | 12k |
| C2 | -0.12057 | 0.50000 | 0.00000 | 6f |
| C3 | 0.50000 | -0.17123 | -0.29200 | 12k |

**Table S2:** Optimized atomic positions of the $C_{60}$-based clathrate structure in the P$m\bar{3}$ simple cubic cell with lattice parameter 6.22Å, using PBE-6-31G(d,p) as implemented in gaussian09.

| atom | x | Y | z | Wyckoff Position |
|---|---|---|---|---|
| C1 | 0.50000 | 0.34890 | -0.14228 | 12k |
| C2 | -0.12129 | 0.50000 | 0.00000 | 6f |
| C3 | 0.50000 | -0.17115 | -0.29187 | 12k |
